# Supplementary material for: Monotone Circuit Lower Bounds from Robust Sunflowers
Source: arXiv:2012.03883 source file (2022-08-05)
Supplement: Supplementary file 1 [file appendix.tex]

\section{Proof of Lemma~\ref{lemma:clique_sunflower}}
Let $\mb U_{n,q} \subseteq [n]$ be a $q$-random subset of $[n]$
(independent of $\mb G(n,p)$).
Let $c_1 \defeq \ln(1/\eps)$ and for $\ell \ge 2$,
let $c_\ell \defeq 2\ln(1/\eps)\sum_{j=1}^{\ell-1}\binom{\ell}{j}c_j$.

\begin{lemma}
    $c_\ell \le \ell!(2\log(1/\eps))^\ell$.
\end{lemma}

\begin{lemma}
    For all $\ell \in \{1,\dots,n\}$ and $S \subseteq
    \binom{[n]}{\ell}$, if $|S| \ge
    c_\ell(1/q)^\ell(1/p)^{\binom{\ell}{2}}$, then there exists
    $B \in \binom{[n]}{<\ell}$ such that
    \[
        \Pr[\ 
            \bigwedge_{A \in S \,:\, B \subseteq A}
            (K_A \nsubseteq \mb G(n,p) \cup K_B \text{ or } 
            A \nsubseteq \mb U_{n,q} \cup B)
        \ ] 
        \le 
        \eps.
    \]
\end{lemma}

\begin{proof}
    By induction on $\ell$. In the base case $\ell=1$, we have
    $B = \emptyset$ and (by independence)
    \[
        \Pr[\ \bigwedge_{A \in S} (K_A \nsubseteq \mb G(n,p) \text{ or } A \nsubseteq \mb U_{n,q})\ ]
        &= 
        \Pr[\ \bigwedge_{A \in S} (A \nsubseteq \mb U_{n,q})\ ]\\
        &=
        \prod_{A \in S} 
        \Pr[\ A \nsubseteq \mb U_{n,q}\ ]\\
        &=
        (1-q)^{|S|}
        \ \ \le\ \ 
        (1-q)^{\ln(1/\eps)/q}
        \ \ \le\ \ 
        e^{-\ln(1/\eps)}
        \ \ =\ \ 
        \eps.
    \]

    Let $\ell \ge 2$. First, consider the case that there
    exists $j \in \{1,\dots,\ell-1\}$ and $B \in
    \binom{[n]}{j}$ such that $$|\{A \in S : B \subseteq A\}|
    \ge c_{\ell-j}(1/qp^j)^{\ell-j}(1/p)^{\binom{\ell-j}{2}}.$$
    Let $T = \{A \setminus B : A \in S \text{ such that } B
\subseteq A\} \subseteq \binom{[n]}{\ell-j}$.  
By the
induction hypothesis, there exists $D \in \binom{[n]
\setminus B}{<\ell -j}$ such that
\[
    \Pr[\ 
        \bigwedge_{C \in T \,:\, D \subseteq C}
        (K_C \nsubseteq \mb G(n,p) \cup K_D \text{ or } 
        C \nsubseteq \mb U_{n,qp^j} \cup D)
    \ ] \le \eps.
\]
We have
\[
    \Pr[\ &\bigwedge_{A \in S \,:\, B \cup D\subseteq A}
        (K_A \nsubseteq \mb G(n,p) \cup K_{B \cup D} \text{ or } 
    A \nsubseteq \mb U_{n,q} \cup B \cup D)\ ]\\
    &=
    \Pr[\ \bigwedge_{C \in T \,:\, D \subseteq C}
        (K_{B \cup C} \nsubseteq \mb G(n,p) \cup K_{B \cup D} \text{ or } 
    B \cup C \nsubseteq \mb U_{n,q} \cup B \cup D)\ ]\\
    &=
    \Pr[\ \bigwedge_{C \in T \,:\, D \subseteq C}
        (K_{B \cup C} \nsubseteq \mb G(n,p) \cup K_{B \cup D} \text{ or } 
    C \nsubseteq \mb U_{n,q} \cup D)\ ]\\
    &=
    \Pr[\ \bigwedge_{C \in T \,:\, D \subseteq C}
        (K_{B \cup C} \nsubseteq \mb G(n,p) \cup K_{B \cup D} \text{ or } 
    C \nsubseteq \mb U_{n,q} \cup D)\ ]\\
    &=
    \Pr[\ \bigwedge_{C \in T \,:\, D \subseteq C}
        (K_C \nsubseteq \mb G(n,p) \cup K_D \text{ or } 
    C \nsubseteq \Big\{v \in \mb U_{n,q} : \{v,w\} \in E(\mb G(n,p)) \text{ for all } w \in B\Big\} \cup D\ ]\\
    &\le
    \Pr[\ \bigwedge_{C \in T \,:\, D \subseteq C}
        (K_C \nsubseteq \mb G(n,p) \cup K_D \text{ or } 
    C \nsubseteq \mb U_{n,qp^j} \cup D\ ]\\
    &\le
    \eps.
\]

Finally, assume that for all $j \in \{1,\dots,\ell-1\}$ and
$B \in \binom{[n]}{j}$, we have $$|\{A \in S : B \subseteq
A\}| \le
c_{\ell-j}(1/qp^j)^{\ell-j}(1/p)^{\binom{\ell-j}{2}}.$$
Let
\[
    \mu &\defeq |S| q^\ell p^{\binom\ell 2},\\
    \Delta &\defeq 
    \sum_{j=1}^{\ell-1} \sum_{(A,A') \in S^2 \,:\, |A \cap A'| = j}
    q^{2\ell-j} p^{2\binom{\ell}{2} - \binom{j}{2}}.
\]
By Janson's inequality,
\[
    \Pr[\ \bigwedge_{A \in S}
        (K_A \nsubseteq \mb G(n,p) \text{ or } 
    A \nsubseteq \mb U_{n,q})\ ]
    &\le
    \exp\left(-
    \frac{\mu^2}{\mu+\Delta}
    \right).
\]
This bound is $\le \exp(- \mu^2/2\Delta)$ when $\Delta \ge
\mu$.

We have $\mu \ge c_\ell$, since $|S| \ge c_\ell (1/q)^\ell
    (1/p)^{\binom\ell 2}$. We also have
    \[
        \Delta &\le
        \sum_{j=1}^{\ell-1} q^{2\ell-j} p^{2\binom{\ell}{2} - \binom{j}{2}} \sum_{B \in \binom{[n]}{j}}
        |\{A \in S : B \subseteq A\}|^2 \\
        &\le
        \sum_{j=1}^{\ell-1} q^{2\ell-j} p^{2\binom{\ell}{2} - \binom{j}{2}} \sum_{B \in \binom{[n]}{j}}
        |\{A \in S : B \subseteq A\}| \cdot c_{\ell-j}(1/q)^{\ell-j}(1/p)^{\binom{\ell-j}{2}}\\
        &=
        q^{\ell}p^{\binom{\ell}{2}} 
        \sum_{j=1}^{\ell-1} c_{\ell-j} \sum_{B \in \binom{[n]}{j}}
        |\{A \in S : B \subseteq A\}|\\
        &=
        q^{\ell}p^{\binom{\ell}{2}}
        \sum_{j=1}^{\ell-1} c_{\ell-j}  
        \sum_{A \in S} \sum_{B \in \binom{A}{j}}
        1\\
        &=
        |S| q^{\ell}p^{\binom{\ell}{2}}
        \sum_{j=1}^{\ell-1}
        \binom{\ell}{j} c_{\ell-j} \\
        &=
        \mu \sum_{j=1}^{\ell-1} \binom{\ell}{j}  c_j.
    \]

    We have
    \[
        \frac{\mu^2}{2\Delta}
        &\ge
        \frac{\mu}{2\sum_{j=1}^{\ell-1} \binom{\ell}{j} c_{\ell-j}}\\
        &=
        \frac{|S| q^\ell p^{\binom\ell 2}}{2\sum_{j=1}^{\ell-1} \binom{\ell}{j} c_{\ell-j} }\\
        &\ge
        \frac{c_\ell}{2\sum_{j=1}^{\ell-1} \binom{\ell}{j} c_{\ell-j}}\\
        &= \ln(1/\eps).
    \]
    By Janson's inequality,
    \[
        \Pr[\ \bigwedge_{A \in S}
            (K_A \nsubseteq \mb G(n,p) \text{ or } 
        A \nsubseteq \mb U_{n,q})\ ]
        &\le
        \exp\left(-\frac{\mu^2}{2\Delta}\right)
        \le
        \eps.
    \]
\end{proof}
